# Supplementary material for: Momentum-Space Cluster Dual Fermion Method
Source: arXiv:1712.03295 ancillary file (2017-12-08)
Supplement: Supplementary file 1 [file supplementary.pdf]

# Supplemental Materials: Momentum-Space Cluster Dual Fermion Method

Sergei Iskakov,[1] Hanna Terletska,[1,2] and Emanuel Gull[1]

[1]*Department of Physics, University of Michigan, Ann Arbor, Michigan 48109, USA*
[2]*Department of Physics, Middle Tennessee State University, Murfreesboro, TN 37132, USA*

(Dated: December 1, 2017)

## I. DUAL ACTION DERIVATIONS

In this section we describe the detailed derivations for the Dual Fermions action formalism. First of all we express the lattice model of $N_{tot}$ sites as a super-lattice by dividing it into $V$ clusters of size $N_c$ each, such that $N_{tot} = VN_c$. The position $i$ of a coordinate in the original lattice is then given as the pair of $\mathbf{I}, \tilde{\mathbf{i}}$, where $\tilde{\mathbf{i}} = 1, \cdots, V$ denotes the position of a cluster in the super-lattice and $\mathbf{I} = 1, \cdots, N_c$ labels sites within each cluster. Then we introduce the separate Fourier transformation for the super-lattice and for clusters as,

$$
\begin{aligned}
c_{\mathbf{I},\tilde{\mathbf{i}},\sigma} &= \frac{1}{\sqrt{V}} \sum_{\tilde{\mathbf{k}}} c_{\mathbf{I},\tilde{\mathbf{k}},\sigma} e^{i\tilde{\mathbf{k}}\tilde{\mathbf{i}}};\\
c_{\mathbf{I},\tilde{\mathbf{i}},\sigma} &= \frac{1}{\sqrt{N_c}} \sum_{\mathbf{K}} c_{\mathbf{K},\tilde{\mathbf{i}},\sigma} e^{i\mathbf{K}\mathbf{I}};\\
c_{\mathbf{K},\tilde{\mathbf{k}},\sigma} &= \frac{1}{\sqrt{V}} \sum_{\tilde{\mathbf{i}}} c_{\mathbf{K},\tilde{\mathbf{i}},\sigma} e^{-i\tilde{\mathbf{k}}\tilde{\mathbf{i}}};\\
c_{\mathbf{K},\tilde{\mathbf{k}},\sigma} &= \frac{1}{\sqrt{N_c}} \sum_{\mathbf{I}} c_{\mathbf{I},\tilde{\mathbf{k}},\sigma} e^{-i\mathbf{K}\mathbf{I}}.
\end{aligned}
\tag{1}
$$

In this case the lattice action is

$$
\begin{aligned}
S = &-\sum_{n,\tilde{\mathbf{k}}} \sum_{\mathbf{K}\mathbf{K}'\sigma} c^*_{\omega_n,\mathbf{K},\tilde{\mathbf{k}},\sigma} \left((i\omega_n + \mu)\delta_{\mathbf{K}\mathbf{K}'} - \hat{\epsilon}_{\mathbf{K}\mathbf{K}'\tilde{\mathbf{k}}}\right) c_{\omega_n,\mathbf{K}',\tilde{\mathbf{k}},\sigma} +\\
&+\frac{U}{N_c V\beta} \sum_{\substack{n,m,l\\ \tilde{\mathbf{k}}\tilde{\mathbf{k}}'\tilde{\mathbf{q}}}} \sum_{\mathbf{K}\mathbf{K}'\mathbf{Q}} c^*_{\omega_n,\mathbf{K},\tilde{\mathbf{k}},\uparrow} c_{\omega_n+\Omega_l,\mathbf{K}+\mathbf{Q},\tilde{\mathbf{k}}+\tilde{\mathbf{q}},\uparrow} c^*_{\omega_m+\Omega_l,\mathbf{K}'+\mathbf{Q},\tilde{\mathbf{k}}'+\tilde{\mathbf{q}},\downarrow} c_{\omega_m,\mathbf{K}',\tilde{\mathbf{k}}',\downarrow}.
\end{aligned}
\tag{2}
$$

Here $\hat{\epsilon}_{\mathbf{K}\mathbf{K}'\tilde{\mathbf{k}}}$ is the reciprocal space representation of the hopping term. This hopping term becomes non-diagonal in reciprocal cluster vectors $K$ and $K'$ due to the breaking of the translational invariance.

$$
\hat{\epsilon}_{\mathbf{K}\mathbf{K}'\tilde{\mathbf{k}}} = \frac{1}{N_c} \sum_{\mathbf{I}\mathbf{J}\tilde{\mathbf{i}}\tilde{\mathbf{j}}} t_{\mathbf{I},\tilde{\mathbf{i}},\mathbf{J},\tilde{\mathbf{j}}} e^{i(\mathbf{K}\mathbf{I} - \mathbf{K}'\mathbf{J} + \tilde{\mathbf{k}}(\tilde{\mathbf{i}} - \tilde{\mathbf{j}}))}.
\tag{3}
$$

In order to express our lattice action in terms of the translationally invariant DCA cluster action, first we need to express interacting term in super-lattice real-space as

$$
\begin{aligned}
&\frac{1}{N_c V\beta} \sum_{\substack{n,m,l\\ \tilde{\mathbf{k}}\tilde{\mathbf{k}}'\tilde{\mathbf{q}}}} \sum_{\mathbf{K}\mathbf{K}'\mathbf{Q}} U c^*_{\omega_n,\mathbf{K},\tilde{\mathbf{k}},\uparrow} c_{\omega_n+\Omega_l,\mathbf{K}+\mathbf{Q},\tilde{\mathbf{k}}+\tilde{\mathbf{q}},\uparrow} c^*_{\omega_m+\Omega_l,\mathbf{K}'+\mathbf{Q},\tilde{\mathbf{k}}'+\tilde{\mathbf{q}},\downarrow} c_{\omega_m,\mathbf{K}',\tilde{\mathbf{k}}',\downarrow} =\\
&= \frac{1}{N_c\beta} \sum_{\substack{n,m,l\\ \tilde{\mathbf{i}}}} \sum_{\mathbf{K}\mathbf{K}'\mathbf{Q}} U c^*_{\omega_n,\mathbf{K},\tilde{\mathbf{i}},\uparrow} c_{\omega_n+\Omega_l,\mathbf{K}+\mathbf{Q},\tilde{\mathbf{i}},\uparrow} c^*_{\omega_m+\Omega_l,\mathbf{K}'+\mathbf{Q},\tilde{\mathbf{i}},\downarrow} c_{\omega_m,\mathbf{K}',\tilde{\mathbf{i}},\downarrow}.
\end{aligned}
\tag{4}
$$

Now we can add and subtract $\sum\limits_{n,\mathbf{K}\tilde{\mathbf{i}}\sigma} c^*_{\omega_n,\mathbf{K},\tilde{\mathbf{i}},\sigma}(\bar{\epsilon}_{\mathbf{K}}+\Delta_{\omega_n\mathbf{K}})c_{\omega_n,\mathbf{K},\tilde{\mathbf{i}},\sigma}$ into lattice action term:

$$S=-\sum_{\substack{n\\ \mathbf{K},\mathbf{K}'\\ \tilde{\mathbf{k}},\sigma}} c^*_{\omega_n,\mathbf{K},\tilde{\mathbf{k}},\sigma}\left((i\omega_n+\mu)\delta_{\mathbf{K}\mathbf{K}'}-\hat{\epsilon}_{\mathbf{K}\mathbf{K}'\tilde{\mathbf{k}}}\right)c_{\omega_n,\mathbf{K}',\tilde{\mathbf{k}},\sigma}+\sum_{\tilde{\mathbf{i}}} S^{(\tilde{\mathbf{i}})}_{int}+$$
$$+\sum_{n\mathbf{K}\tilde{\mathbf{i}}\sigma} c^*_{\omega_n,\mathbf{K},\tilde{\mathbf{i}},\sigma}(\bar{\epsilon}_{\mathbf{K}}+\Delta_{\omega_n\mathbf{K}})c_{\omega_n,\mathbf{K},\tilde{\mathbf{i}},\sigma}-\sum_{n\mathbf{K}\tilde{\mathbf{i}}\sigma} c^*_{\omega_n,\mathbf{K},\tilde{\mathbf{i}},\sigma}(\bar{\epsilon}_{\mathbf{K}}+\Delta_{\omega_n\mathbf{K}})c_{\omega_n,\mathbf{K},\tilde{\mathbf{i}},\sigma}. \tag{5}$$

Since DCA cluster quantities are independent of cluster position in the super lattice we can transform the last term into super-lattice reciprocal space:

$$S=-\sum_{n\mathbf{K}\tilde{\mathbf{i}}\sigma} c^*_{\omega_n,\mathbf{K},\tilde{\mathbf{i}},\sigma}\left(i\omega_n+\mu-\bar{\epsilon}_{\mathbf{K}}-\Delta_{\omega_n\mathbf{K}}\right)c_{\omega_n,\mathbf{K},\tilde{\mathbf{i}},\sigma}+$$
$$+\sum_{\tilde{\mathbf{i}}} S^{(\tilde{\mathbf{i}})}_{int}-\sum_{n\mathbf{K}\mathbf{K}'\tilde{\mathbf{k}}\sigma} c^*_{\omega_n,\mathbf{K},\tilde{\mathbf{k}},\sigma}((\Delta_{\omega_n\mathbf{K}}+\bar{\epsilon}_{\mathbf{K}})\delta_{\mathbf{K}\mathbf{K}'}-\hat{\epsilon}_{\mathbf{K}\mathbf{K}'\tilde{\mathbf{k}}})c_{\omega_n,\mathbf{K}',\tilde{\mathbf{k}},\sigma}=$$
$$=\sum_{\tilde{\mathbf{i}}} S^{(\tilde{\mathbf{i}})}_{c}-\sum_{n\mathbf{K}\mathbf{K}'\tilde{\mathbf{k}}\sigma} c^*_{\omega_n,\mathbf{K},\tilde{\mathbf{k}},\sigma}((\Delta_{\omega_n\mathbf{K}}+\bar{\epsilon}_{\mathbf{K}})\delta_{\mathbf{K}\mathbf{K}'}-\hat{\epsilon}_{\mathbf{K}\mathbf{K}'\tilde{\mathbf{k}}})c_{\omega_n,\mathbf{K}',\tilde{\mathbf{k}},\sigma}. \tag{6}$$

We then perform a Hubbard-Stratonovich transformation, defined as

$$e^{c^*_\alpha a^{-1}_{\alpha\beta}c_\beta}=\frac{1}{\det(b_\alpha a_{\alpha\beta}b_\beta)}\int e^{-\xi^*_\alpha b_\alpha a_{\alpha\beta}b_\beta\xi_\beta+\xi^*_\alpha b_\alpha c_\alpha+c^*_\alpha b_\alpha\xi_\alpha}\mathcal{D}[\xi^*_{\tilde{\mathbf{k}}}\xi_{\tilde{\mathbf{k}}}], \tag{7}$$

choosing $a_{\alpha\beta}=((\Delta_{\omega_n\mathbf{K}}+\bar{\epsilon}_{\mathbf{K}})\delta_{\mathbf{K}\mathbf{K}'}-\hat{\epsilon}_{\mathbf{K}\mathbf{K}'\tilde{\mathbf{k}}})^{-1}$, and $b$ as an arbitrary function of $\omega_n$, $\mathbf{K}$ and $\sigma$. And we can now express lattice action in lattice fermion operators and dual fermion operators:

$$S=\sum_{\tilde{\mathbf{i}}} S^{(\tilde{\mathbf{i}})}_{c}+\sum_{KK'\tilde{\mathbf{k}}}\xi^*_{K\tilde{\mathbf{k}}}b_K\frac{1}{((\Delta_{\omega_n\mathbf{K}}+\bar{\epsilon}_{\mathbf{K}})\delta_{\mathbf{K}\mathbf{K}'}-\hat{\epsilon}_{\mathbf{K}\mathbf{K}'\tilde{\mathbf{k}}})}b_{K'}\xi_{K'\tilde{\mathbf{k}}}-\sum_{K\tilde{\mathbf{k}}}(\xi^*_{K\tilde{\mathbf{k}}}b_Kc_{K\tilde{\mathbf{k}}}+c^*_{K\tilde{\mathbf{k}}}b_K\xi_{K\tilde{\mathbf{k}}})+ln(Z_f)=$$
$$=\sum_{\tilde{\mathbf{i}}} S^{(\tilde{\mathbf{i}})}_{c}-\sum_{K\tilde{\mathbf{i}}}(\xi^*_{K\tilde{\mathbf{i}}}b_Kc_{K\tilde{\mathbf{i}}}+c^*_{K\tilde{\mathbf{i}}}b_K\xi_{K\tilde{\mathbf{i}}})+\sum_{KK'\tilde{\mathbf{k}}}\xi^*_{K\tilde{\mathbf{k}}}b_K\frac{1}{((\Delta_{\omega_n\mathbf{K}}+\bar{\epsilon}_{\mathbf{K}})\delta_{\mathbf{K}\mathbf{K}'}-\hat{\epsilon}_{\mathbf{K}\mathbf{K}'\tilde{\mathbf{k}}})}b_{K'}\xi_{K'\tilde{\mathbf{k}}}, \tag{8}$$

$Z_f=\frac{1}{\det(bab)}$ is constant and can be omitted. Since $b=b(K)$, we can transform the last term in the first line into superlattice real space and integrate out the lattice fermion operators for each super lattice site $\tilde{\mathbf{i}}$ separately:

$$\int e^{-S^{(\tilde{\mathbf{i}})}_c}e^{\sum\limits_K(\xi^*_{K\tilde{\mathbf{i}}}b_Kc_{K\tilde{\mathbf{i}}}+c^*_{K\tilde{\mathbf{i}}}b_K\xi_{K\tilde{\mathbf{i}}})}\mathcal{D}\left[c^*_{\tilde{\mathbf{i}}},c_{\tilde{\mathbf{i}}}\right]=\mathcal{Z}_c\left\langle e^{\sum\limits_K(\xi^*_{K\tilde{\mathbf{i}}}b_Kc_{K\tilde{\mathbf{i}}}+c^*_{K\tilde{\mathbf{i}}}b_K\xi_{K\tilde{\mathbf{i}}})}\right\rangle_c \tag{9}$$

Perform the Taylor series expansion for the exponent in the angle brackets:

$$e^{\sum\limits_K(\xi^*_{K\tilde{\mathbf{i}}}b_Kc_{K\tilde{\mathbf{i}}}+c^*_{K\tilde{\mathbf{i}}}b_K\xi_{K\tilde{\mathbf{i}}})}=\sum_{n=0}^{\infty}\frac{1}{n!}(\sum_K(\xi^*_{K\tilde{\mathbf{i}}}b_Kc_{K\tilde{\mathbf{i}}}+c^*_{K\tilde{\mathbf{i}}}b_K\xi_{K\tilde{\mathbf{i}}}))^n \tag{10}$$

Since $\langle\ldots\rangle_c$ is nonzero only for even number of $c^*c$ pairs, Eq. 10 can be simplified:

$$(10)=\sum_{n\in even}\frac{1}{n!}(\sum_K(\xi^*_{K\tilde{\mathbf{i}}}b_Kc_{K\tilde{\mathbf{i}}}+c^*_{K\tilde{\mathbf{i}}}b_K\xi_{K\tilde{\mathbf{i}}}))^n=\sum_{n\in even}\mathcal{F}_n. \tag{11}$$

And express $\mathcal{F}_n$ with the following restrictions $n \in \{0,2,4\}$:

$$\mathcal{F}_0 = 1 \tag{12}$$

$$\begin{aligned}
\mathcal{F}_2 &= \frac{1}{2}\sum_{K_1K_2} c_{K_1}\xi^*_{K_1}b_{K_1}b_{K_2}c^*_{K_2}\xi_{K_2} + c^*_{K_1}\xi_{K_1}b_{K_1}b_{K_2}c_{K_2}\xi^*_{K_2} + b_{K_1}c_{K_1}\xi^*_{K_1}b_{K_2}c_{K_2}\xi^*_{K_2} + b_{K_1}c^*_{K_1}\xi_{K_1}b_{K_2}c^*_{K_2}\xi_{K_2} = \\
&= \left|\begin{smallmatrix}\langle cc\rangle=0\\ \langle c^*c^*\rangle=0\end{smallmatrix}\right| = \frac{1}{2}\sum_{K_1K_2} c_{K_1}c^*_{K_2}b_{K_1}b_{K_2}\xi^*_{K_1}\xi_{K_2} + c_{K_2}c^*_{K_1}b_{K_1}b_{K_2}\xi^*_{K_2}\xi_{K_1} = \sum_{K_1K_2} c_{K_1}c^*_{K_2}b_{K_1}b_{K_2}\xi^*_{K_1}\xi_{K_2} = \\
&= \sum_{K_1K_2}\sum_{I_1I_2}\int \frac{1}{\sqrt{\beta N_c}}c_{I_1\tau_1}\frac{1}{\sqrt{\beta N_c}}c^*_{I_2\tau_2}e^{i\sum_{m=1}^{2}(-1)^m(\tau_m\omega_m+I_m\mathbf{K_m})}d\tau_1 d\tau_2 b_{K_1}b_{K_2}\xi^*_{K_1}\xi_{K_2}
\end{aligned} \tag{13}$$

$$\begin{aligned}
\mathcal{F}_4 &= \frac{1}{4!}\left[\sum_{K_1K_2} 2c_{K_1}c^*_{K_2}b_{K_1}b_{K_2}\xi_{K_2}\xi^*_{K_1} + b_{K_1}c_{K_1}\xi^*_{K_1}b_{K_2}c_{K_2}\xi^*_{K_2} + b_{K_1}c^*_{K_1}\xi_{K_1}b_{K_2}c^*_{K_2}\xi_{K_2}\right]^2 = \left|\begin{smallmatrix}\langle cccc\rangle=0\\ \langle cccc^*\rangle=0\\ \langle cc^*c^*c^*\rangle=0\\ \langle c^*c^*c^*c^*\rangle=0\end{smallmatrix}\right| = \\
&= \frac{1}{4}\sum_{K_1K_2K_3K_4} c_{K_1}c_{K_3}c^*_{K_2}c^*_{K_4}b_{K_1}b_{K_2}b_{K_3}b_{K_4}\xi_{K_2}\xi_{K_4}\xi^*_{K_1}\xi^*_{K_3} = \\
&= \frac{1}{4}\sum_{K_1K_2K_3K_4}\sum_{I_1I_2I_3I_4}\int \frac{1}{\sqrt{\beta N_c}}c_{I_1\tau_1}\frac{1}{\sqrt{\beta N_c}}c_{I_3\tau_3}\frac{1}{\sqrt{\beta N_c}}c^*_{I_2\tau_2}\frac{1}{\sqrt{\beta N_c}}c^*_{I_4\tau_4}e^{i\sum_{m=1}^{4}(-1)^m(\tau_m\omega_m+I_m\mathbf{K_m})}d\tau_1 d\tau_2 d\tau_3 d\tau_4\times \\
&\times b_{K_1}b_{K_2}b_{K_3}b_{K_4}\xi_{K_2}\xi_{K_4}\xi^*_{K_1}\xi^*_{K_3}.
\end{aligned} \tag{14}$$

Using the definitions $G^c_{I_1\tau_1I_2\tau_2} = -\langle c_{I_1\tau_1}c^*_{I_2\tau_2}\rangle_c$ and $G^{4,c}_{I_1\tau_1,I_2\tau_2,I_3\tau_3,I_4\tau_4} = \langle c_{I_1\tau_1}c_{I_2\tau_2}c^*_{I_3\tau_3}c^*_{I_4\tau_4}\rangle_c$, this leads to the following:

$$\begin{aligned}
\left\langle \sum_{n\in even}\mathcal{F}_n\right\rangle_c &= 1 + \sum_{K_1K_2}\frac{1}{\beta N_c}\sum_{I_1I_2}\int \left\langle c_{I_1\tau_1}c^*_{I_2\tau_2}\right\rangle_c e^{i\sum\limits_{m=1}^{2}(-1)^m(\tau_m\omega_m+I_m\mathbf{K_m})}d\tau_1 d\tau_2 b_{K_1}b_{K_2}\xi^*_{K_1}\xi_{K_2} + \\
&+ \frac{1}{4}\sum_{K_1K_2K_3K_4}\sum_{I_1I_2I_3I_4}\int \frac{1}{\beta^2N_c^2}\left\langle c_{I_1\tau_1}c_{I_3\tau_3}c^*_{I_2\tau_2}c^*_{I_4\tau_4}\right\rangle_c e^{i\sum\limits_{m=1}^{4}(-1)^m(\tau_m\omega_m+I_m\mathbf{K_m})}d\tau_1 d\tau_2 d\tau_3 d\tau_4\times \\
&\times b_{K_1}b_{K_2}b_{K_3}b_{K_4}\xi_{K_2}\xi_{K_4}\xi^*_{K_1}\xi^*_{K_3} = \\
&= 1 - \sum_{K_1K_2}\frac{1}{\beta N_c}\sum_{I_1I_2}\int G^c_{I_1\tau_1I_2\tau_2}e^{i\sum\limits_{m=1}^{2}(-1)^m(\tau_m\omega_m+I_m\mathbf{K_m})}d\tau_1 d\tau_2 b_{K_1}b_{K_2}\xi^*_{K_1}\xi_{K_2} + \\
&+ \frac{1}{4}\sum_{K_1K_2K_3K_4}\sum_{I_1I_2I_3I_4}\int \frac{1}{\beta^2N_c^2}G^{4,c}_{I_1\tau_1,I_2\tau_2,I_3\tau_3,I_4\tau_4}e^{i\sum\limits_{m=1}^{4}(-1)^m(\tau_m\omega_m+I_m\mathbf{K_m})}d\tau_1 d\tau_2 d\tau_3 d\tau_4\times \\
&\times b_{K_1}b_{K_2}b_{K_3}b_{K_4}\xi_{K_2}\xi_{K_4}\xi^*_{K_1}\xi^*_{K_3}
\end{aligned} \tag{15}$$

Implying the momentum conservation[1] and performing Fourier transform to frequecy-momentum domain we will now get:

$$(15) = 1 - \sum_K G^c_K b_K b_K \xi^*_K \xi_K \delta_{K_1,K_2} + \frac{1}{\beta N_c}\frac{1}{4}\sum_{KK'Q} G^{4,c}_{K,K'+Q,K',K+Q} b_K b_{K+Q} b_{K'+Q} b_{K'} \xi_{K'}\xi_{K+Q}\xi^*_K\xi^*_{K'+Q}\delta_{K_1+K_2,K_3+K_4} \tag{16}$$

The result of the integrating out the lattice fermions should have the following form:

$$e^{\sum\limits_K \xi^*_{K\tilde{\mathbf{i}}}b_K\xi_{K\tilde{\mathbf{i}}} - V\left[\xi^*_{\tilde{\mathbf{i}}},\xi_{\tilde{\mathbf{i}}}\right]}, \tag{17}$$

where $V\left[\xi^*_{\tilde{\mathbf{i}}},\xi_{\tilde{\mathbf{i}}}\right] = \sum_{n\in even}\alpha^{(n)}\prod\limits_{i=1}^{n-1}\xi^*_{i1}\xi_{i2}$ is a dual potential. By performing the Taylor series expansion of the Eq.

17 and keeping only the terms with 4 or less dual operators we get:

$$(17) = 1 + (\sum_K \xi^*_{K\tilde{\mathbf{i}}} b_K \xi_{K\tilde{\mathbf{i}}} + \sum_{K_1K_2} \alpha^{(2)} \xi^*_{K_1}\xi_{K_2} + \sum_{K_1K_2K_3K_4} \alpha^{(4)} \xi^*_{K_1}\xi^*_{K_2}\xi_{K_3}\xi_{K_4}) + \frac{1}{2}(\sum_K\sum_{K'} b_K b_{K'} \xi^*_{K\tilde{\mathbf{i}}}\xi^*_{K'\tilde{\mathbf{i}}}\xi_{K\tilde{\mathbf{i}}}\xi_{K'\tilde{\mathbf{i}}}) =$$

$$= 1 + (\sum_K \xi^*_{K\tilde{\mathbf{i}}} b_K \xi_{K\tilde{\mathbf{i}}} + \sum_{K_1K_2} \alpha^{(2)} \xi^*_{K_1}\xi_{K_2} +$$

$$+ \sum_{K_1K_2K_3K_4} [\alpha^{(4)} + \frac{1}{4}(b_{K_1}b_{K_2}\delta_{K_1,K_4}\delta_{K_2,K_3} - b_{K_1}b_{K_2}\delta_{K_1,K_3}\delta_{K_2,K_4})]\xi^*_{K_1}\xi^*_{K_2}\xi_{K_3}\xi_{K_4}) \tag{18}$$

Until this point $b_K$ remains a free parameter, to simplify the form of dual potential it should be chosen in a way to eliminate $\alpha^{(2)}$:

$$\sum_K \xi^*_{K\tilde{\mathbf{i}}} b_K \xi_{K\tilde{\mathbf{i}}} + \alpha^{(2)} \sum_{K_1K_2} \xi^*_{K_1}\xi_{K_2} = -\sum_K G^c_K b_K b_K \xi^*_K \xi_K \Rightarrow -G^c_K b_K b_K = b_K \Rightarrow b_K = -(G^c_K)^{-1}, \tag{19}$$

that gives us $\alpha^{(2)} = 0$ and $\alpha^{(4)}$ can be described as follows:

$$\alpha^{(4)} = \frac{1}{4}\frac{1}{\beta N_c}\sum_{KK'Q}\left[\frac{G^{4,c}_{KK'Q}}{G^c_K G^c_{K'+Q} G^c_{K'} G^c_{K+Q}} + \frac{\beta N_c}{G^c_K G^c_{K+Q}} - \frac{\beta N_c}{G^c_K G^c_{K'}}\right] =$$

$$= \frac{1}{4}\frac{1}{\beta N_c}\sum_{KK'Q}\left[\frac{G^{4,c}_{KK'Q} + \beta N_c G^c_K G^c_{K'} - \beta N_c G^c_K G^c_{K+Q}}{G^c_K G^c_{K'+Q} G^c_{K'} G^c_{K+Q}}\right] = \frac{1}{4}\frac{1}{\beta N_c}\sum_{KK'Q}\gamma_{KK'Q} \tag{20}$$

The original lattice action problem now can be expressed using only dual operators:

$$S[\xi^*,\xi] = \sum_{n\mathbf{K}\mathbf{K}'\tilde{\mathbf{k}}\sigma} \xi^*_{\omega_n,\mathbf{K},\tilde{\mathbf{k}},\sigma} G^{(c)^{-1}}_K \left[((\Delta_{\omega_n\mathbf{K}} + \bar{\epsilon}_{\mathbf{K}})_{\delta_{\mathbf{K}\mathbf{K}'}} - \hat{\epsilon}_{\mathbf{K}\mathbf{K}'\tilde{\mathbf{k}}})\right]^{-1} G^{(c)^{-1}}_{K'} \xi_{\omega_n,\mathbf{K}',\tilde{\mathbf{k}},\sigma} +$$

$$+\sum_{\tilde{\mathbf{i}}}\left(\sum_{n\mathbf{K}\sigma}\xi^*_{\omega_n,\mathbf{K},\tilde{\mathbf{i}},\sigma} G^{(c)^{-1}}_K \xi_{\omega_n,\mathbf{K},\tilde{\mathbf{i}},\sigma} + V\left[\xi^*_{\tilde{\mathbf{i}}},\xi_{\tilde{\mathbf{i}}}\right]\right) = -\sum_{n\mathbf{K}\mathbf{K}'\tilde{\mathbf{k}}\sigma} \xi^*_{\omega_n,\mathbf{K},\tilde{\mathbf{k}},\sigma} \tilde{G}^{(0)}_{\omega_n\mathbf{K}\mathbf{K}'\tilde{\mathbf{k}}\sigma}{}^{-1} \xi_{\omega_n,\mathbf{K}',\tilde{\mathbf{k}},\sigma} + \sum_{\tilde{\mathbf{i}}} V\left[\xi^*_{\tilde{\mathbf{i}}},\xi_{\tilde{\mathbf{i}}}\right], \tag{21}$$

where $\tilde{G}^{(0)}_{\omega_n\mathbf{K}\mathbf{K}'\tilde{\mathbf{k}}\sigma} = -G^{(c)}_K\left[G^{(c)}_{K'} + ((\Delta_{\omega_n\mathbf{K}} + \bar{\epsilon}_{\mathbf{K}})_{\delta_{\mathbf{K}\mathbf{K}'}} - \hat{\epsilon}_{\mathbf{K}\mathbf{K}'\tilde{\mathbf{k}}})^{-1}\right]^{-1} G^{(c)}_{K'}$ is a bare dual Green's function.

## II. SELF-ENERGY EVALUATION

The next step for consistent derivations is the construction of the diagrammatic perturbation series. For this case we will introduce dual Luttinger-Ward functional by the following:

$$\tilde{\Phi} = \int_{\Phi} e^{-\tilde{S}^{(0)}} e^{-\sum_{\tilde{\mathbf{i}}} V[\xi^*_{\tilde{\mathbf{i}}},\xi_{\tilde{\mathbf{i}}}]} \mathcal{D}[\xi^*\xi] = \int_{\Phi}\prod_n \frac{1}{n!}\sum_{\tilde{\mathbf{i}}_n}\sum_{KK'Q}\frac{1}{4}\frac{1}{\beta N_c}\gamma^{(4)}_{KK'Q}\xi^*_{\tilde{\mathbf{i}}_n,K'}\xi^*_{\tilde{\mathbf{i}}_n,K+Q}\xi_{\tilde{\mathbf{i}}_n,K}\xi_{\tilde{\mathbf{i}}_n,K'+Q}\mathcal{D}[\xi^*\xi], \tag{22}$$

where $\tilde{S}^{(0)} = \sum_{\omega_n\mathbf{K}\mathbf{K}'\tilde{\mathbf{k}}\sigma}\xi^*_{\omega_n\mathbf{K}\mathbf{K}'\tilde{\mathbf{k}}\sigma}\tilde{G}^{(0)}_{\omega_n\mathbf{K}\tilde{\mathbf{k}}\sigma}{}^{-1}\xi_{\omega_n\mathbf{K}\tilde{\mathbf{k}}\sigma}$ is dual non-interacting part of the action. Since the bare dual Green's function can be defined as $\int e^{-\tilde{S}^{(0)}}\xi^*_{\mathbf{K}\tilde{\mathbf{k}}}\xi_{\mathbf{K}'\tilde{\mathbf{k}}}\mathcal{D}[\xi^*\xi] = \tilde{G}^{(0)}_{\mathbf{K}\mathbf{K}'\tilde{\mathbf{k}}}$. we can rewrite the perturbation series by means of dual Green's. For this reason we need to perform a Fourier transformation for dual operators. Since we have a broken translational invariance in cluster the first order diagram will also contribute. And the self-energy can be defined as functional derivitive $\tilde{\Sigma} = \frac{\delta\tilde{\Phi}[\tilde{G}]}{\delta\tilde{G}}$. For second order contribution into the $\tilde{\Sigma}$ diagram we will be given as:

$$\delta\tilde{\Sigma}^{(2)}_{\tilde{\mathbf{k}}\mathbf{K}_1\mathbf{K}_2\omega_n} = -\frac{1}{N_c^2V^2\beta^2}\frac{1}{2}\sum_{\substack{ml\\ \mathbf{K}'_1\mathbf{Q}_1\\ \mathbf{K}'_2\mathbf{Q}_2}}\gamma^{(4)}_{\substack{\omega_n\omega_m\Omega_l\\ \mathbf{K}_1\mathbf{K}'_1\mathbf{Q}_1}}\gamma^{(4)}_{\substack{\omega_m\omega_n\Omega_l\\ \mathbf{K}_2\mathbf{K}'_2\mathbf{Q}_2}}\sum_{\tilde{\mathbf{k}}'\tilde{\mathbf{q}}}\tilde{G}^{(0)}_{\omega_m,\mathbf{K}'_1,\mathbf{K}'_2,\tilde{\mathbf{k}}'}\tilde{G}^{(0)}_{\omega_m+\Omega_l,\mathbf{K}'_1+\mathbf{Q}_1,\mathbf{K}'_2+\mathbf{Q}_2,\tilde{\mathbf{k}}'+\tilde{\mathbf{q}}}\tilde{G}^{(0)}_{\omega_m+\Omega_l,\mathbf{K}_1+\mathbf{Q}_1,\mathbf{K}_2+\mathbf{Q}_2,\tilde{\mathbf{k}}+\tilde{\mathbf{q}}} \tag{23}$$

The next step is to derive the relation between dual self-energy, $\tilde{\Sigma}$, and lattice one. For this purpose lets start our consideration from the Eq. 8 and keep $ln(Z_f)$ in action. In this case the partition function can be expressed as

$$\mathcal{Z} = \int e^{-S[c^*,c]}\mathcal{D}[c^*,c] = Z_f \int e^{-S[c^*,c,\xi^*,\xi]}\mathcal{D}[c^*,c,\xi^*,\xi]. \tag{24}$$

Then we can obtain lattice Green's function from the functional derivitive of the partition function with respect to dispersion part of the action, $h_{n\mathbf{K}\mathbf{K}'\tilde{\mathbf{k}}} = \hat{\epsilon}_{\mathbf{K}\mathbf{K}'\tilde{\mathbf{k}}}\mathbb{1}_n$:

$$\begin{aligned}
-\frac{\delta\mathcal{Z}[h]}{\delta h_{n\mathbf{K}'\mathbf{K}\tilde{\mathbf{k}}}} =& -\frac{\delta}{\delta h_{n\mathbf{K}'\mathbf{K}\tilde{\mathbf{k}}}}\int e^{\sum_{m\hat{\mathbf{K}}\hat{\mathbf{K}}'\hat{\tilde{k}}\sigma} c^*_{\omega_m,\hat{\mathbf{K}},\hat{\tilde{k}},\sigma}\left((i\omega_m+\mu)\delta_{\hat{\mathbf{K}}\hat{\mathbf{K}}'}-\hat{\epsilon}_{\hat{\mathbf{K}}\hat{\mathbf{K}}'\hat{\tilde{k}}}\right)c_{\omega_m,\hat{\mathbf{K}}',\hat{\tilde{k}},\sigma}-S_{int}}\mathcal{D}[c^*,c] = \\
=&\delta_{n,m}\int\sum_{n\hat{\mathbf{K}}\hat{\mathbf{K}}'\hat{\tilde{k}}\sigma} c^*_{\omega_n,\hat{\mathbf{K}},\hat{\tilde{k}},\sigma}\frac{\delta\hat{\epsilon}_{\hat{\mathbf{K}}\hat{\mathbf{K}}'\hat{\tilde{k}}}}{\delta\hat{\epsilon}_{\mathbf{K}'\mathbf{K}\tilde{\mathbf{k}}}}c_{\omega_n,\hat{\mathbf{K}}',\hat{\tilde{k}},\sigma}e^{-S[c^*,c]}\mathcal{D}[c^*,c] = \\
=&\delta_{n,m}\delta_{\hat{\mathbf{K}},\mathbf{K}'}\delta_{\hat{\mathbf{K}}',\mathbf{K}}\delta_{\hat{\tilde{k}},\tilde{\mathbf{k}}}\int c^*_{\omega_m,\hat{\mathbf{K}},\hat{\tilde{k}},\sigma}c_{\omega_m,\hat{\mathbf{K}}',\hat{\tilde{k}},\sigma}e^{-S[c^*,c]}\mathcal{D}[c^*,c] = \mathcal{Z}G_{\omega_n\mathbf{K}\mathbf{K}'\tilde{\mathbf{k}}}
\end{aligned} \tag{25}$$

On the next step we apply functional derivative over $h$ to the right-hand side of the Eq. 24 and divide it by $\mathcal{Z}$ and :

$$\frac{1}{\mathcal{Z}}\frac{\delta}{\delta h_{n\mathbf{K}'\mathbf{K}\tilde{\mathbf{k}}}}Z_f\int e^{-S[c^*,c,\xi^*,\xi]}\mathcal{D}[c^*,c,\xi^*,\xi] = \frac{1}{\mathcal{Z}}\left[\frac{\delta Z_f}{\delta h_{n\mathbf{K}'\mathbf{K}\tilde{\mathbf{k}}}}\int e^{-S[c^*,c,\xi^*,\xi]}\mathcal{D}[c^*,c,\xi^*,\xi] + Z_f\frac{\delta\int e^{-S[c^*,c,\xi^*,\xi]}\mathcal{D}[c^*,c,\xi^*,\xi]}{\delta h_{n\mathbf{K}'\mathbf{K}\tilde{\mathbf{k}}}}\right]. \tag{26}$$

Consider the first term using the fact that $Z_f = \det(G_{K'}\left((\Delta_{\omega_n\mathbf{K}}+\bar{\epsilon}_{\mathbf{K}})_{\delta_{\mathbf{K}\mathbf{K}'}} - \hat{\epsilon}_{\mathbf{K}'\mathbf{K}\tilde{\mathbf{k}}}\right)G_K)$ and Jacobi's formula :

$$\begin{aligned}
\frac{\delta Z_f}{\delta h_{n\mathbf{K}'\mathbf{K}\tilde{\mathbf{k}}}} =& Z_f Tr\left[G^{-1}_{\hat{K}'}\left((\Delta_{\omega_n\hat{\mathbf{K}}}+\bar{\epsilon}_{\hat{\mathbf{K}}})_{\delta_{\hat{\mathbf{K}}\hat{\mathbf{K}}'}} - \hat{\epsilon}_{\hat{\mathbf{K}}\hat{\mathbf{K}}'\hat{\tilde{k}}}\right)^{-1}G^{-1}_{\hat{K}}\frac{\delta(G_{\hat{K}}\left((\Delta_{\omega_n\hat{\mathbf{K}}}+\bar{\epsilon}_{\hat{\mathbf{K}}})_{\delta_{\hat{\mathbf{K}}\hat{\mathbf{K}}'}} - \hat{\epsilon}_{\hat{\mathbf{K}}\hat{\mathbf{K}}'\hat{\tilde{k}}}\right)G_{\hat{K}'})}{\delta h_{n\mathbf{K}'\mathbf{K}\tilde{\mathbf{k}}}}\right] = \\
=& -Z_f\left((\Delta_{\omega_n\mathbf{K}}+\bar{\epsilon}_{\mathbf{K}})_{\delta_{\mathbf{K}\mathbf{K}'}} - \hat{\epsilon}_{\mathbf{K}\mathbf{K}'\tilde{\mathbf{k}}}\right)^{-1}
\end{aligned} \tag{27}$$

Now lets consider the second term in the Eq. 26:

$$\begin{aligned}
&Z_f\frac{\delta\int e^{-S[c^*,c,\xi^*,\xi]}\mathcal{D}[c^*,c,\xi^*,\xi]}{\delta h_{n\mathbf{K}'\mathbf{K}\tilde{\mathbf{k}}}} = \\
&=Z_f\frac{\delta}{\delta h_{n\mathbf{K}'\mathbf{K}\tilde{\mathbf{k}}}}\int e^{-S_{rest}-\sum_{m\hat{\mathbf{K}}\hat{\mathbf{K}}'\tilde{\mathbf{k}}\sigma}\xi^*_{\omega_m,\hat{\mathbf{K}},\tilde{\mathbf{k}},\sigma}G^{-1}_{\hat{K}}((\Delta_{\omega_n\hat{\mathbf{K}}}+\bar{\epsilon}_{\hat{\mathbf{K}}})_{\delta_{\hat{\mathbf{K}}\hat{\mathbf{K}}'}}-\hat{\epsilon}_{\hat{\mathbf{K}}\hat{\mathbf{K}}'\hat{\tilde{k}}})^{-1}G^{-1}_{\hat{K}'}\xi_{\omega_m,\hat{\mathbf{K}}',\tilde{\mathbf{k}},\sigma}}\mathcal{D}[c^*,c,\xi^*,\xi] = \\
&=-Z_f\delta_{n,m}\int\frac{\delta}{\delta h_{n\mathbf{K}'\mathbf{K}\tilde{\mathbf{k}}}}\left[\xi^*_{\omega_m,\hat{\mathbf{K}},\hat{\tilde{k}},\sigma}G^{-1}_{\hat{K}}((\Delta_{\omega_n\hat{\mathbf{K}}}+\bar{\epsilon}_{\hat{\mathbf{K}}})_{\delta_{\hat{\mathbf{K}}\hat{\mathbf{K}}'}}-\hat{\epsilon}_{\hat{\mathbf{K}}\hat{\mathbf{K}}'\hat{\tilde{k}}})^{-1}G^{-1}_{\hat{K}'}\xi_{\omega_m,\hat{\mathbf{K}}',\hat{\tilde{k}},\sigma}\right]e^{-S}\mathcal{D}[c^*,c,\xi^*,\xi] = \\
&=Z_f\delta_{m,n}\delta_{\tilde{\mathbf{k}},\hat{\tilde{k}}}\left[\left((\Delta_{\omega_n\mathbf{K}}+\bar{\epsilon}_{\mathbf{K}})_{\delta_{\mathbf{K}\mathbf{K}^{(2)}}}-\hat{\epsilon}_{\mathbf{K}\mathbf{K}^{(2)}\tilde{\mathbf{k}}}\right)^{-1}G^{-1}_{\omega_n\mathbf{K}^{(2)}}\right]\int\xi_{\omega_m,\hat{\mathbf{K}}^2,\tilde{\mathbf{k}},\sigma}\xi^*_{\omega_m,\hat{\mathbf{K}}^3,\tilde{\mathbf{k}},\sigma}e^{-S}\mathcal{D}[c^*,c,\xi^*,\xi]\times \\
&\times\left[G^{-1}_{\omega_n\mathbf{K}^{(3)}}\left((\Delta_{\omega_n\mathbf{K}'}+\bar{\epsilon}_{\mathbf{K}'})_{\delta_{\mathbf{K}^{(3)}\mathbf{K}'}}-\hat{\epsilon}_{\mathbf{K}^{(3)}\mathbf{K}'\tilde{\mathbf{k}}}\right)^{-1}\right] = \\
&=-\mathcal{Z}\left[\left((\Delta_{\omega_n\mathbf{K}}+\bar{\epsilon}_{\mathbf{K}})_{\delta_{\mathbf{K}\mathbf{K}^{(2)}}}-\hat{\epsilon}_{\mathbf{K}\mathbf{K}^{(2)}\tilde{\mathbf{k}}}\right)^{-1}G^{-1}_{\omega_n\mathbf{K}^{(2)}}\right]\tilde{G}_{\omega_n\mathbf{K}^{(2)}\mathbf{K}^{(3)}\tilde{\mathbf{k}}}\left[G^{-1}_{\omega_n\mathbf{K}^{(3)}}\left((\Delta_{\omega_n\mathbf{K}'}+\bar{\epsilon}_{\mathbf{K}'})_{\delta_{\mathbf{K}^{(3)}\mathbf{K}'}}-\hat{\epsilon}_{\mathbf{K}^{(3)}\mathbf{K}'\tilde{\mathbf{k}}}\right)^{-1}\right]
\end{aligned} \tag{28}$$

we can finally get the relation between dual and lattice Green's functions:

$$\begin{aligned}
\mathbf{G}_{\omega_n\mathbf{K}\mathbf{K}'\tilde{\mathbf{k}}} = \left((\Delta_{\omega_n\mathbf{K}}+\bar{\epsilon}_{\mathbf{K}})_{\delta_{\mathbf{K}\mathbf{K}'}}-\hat{\epsilon}_{\mathbf{K}\mathbf{K}'\tilde{\mathbf{k}}}\right)^{-1} + \left[\left((\Delta_{\omega_n\mathbf{K}}+\bar{\epsilon}_{\mathbf{K}})_{\delta_{\mathbf{K}\mathbf{K}^{(2)}}}-\hat{\epsilon}_{\mathbf{K}\mathbf{K}^{(2)}\tilde{\mathbf{k}}}\right)^{-1}G^{-1}_{\omega_n\mathbf{K}^{(2)}}\right]\tilde{G}_{\omega_n\mathbf{K}^{(2)}\mathbf{K}^{(3)}\tilde{\mathbf{k}}}\times \\
\times\left[G^{-1}_{\omega_n\mathbf{K}^{(3)}}\left((\Delta_{\omega_n\mathbf{K}'}+\bar{\epsilon}_{\mathbf{K}'})_{\delta_{\mathbf{K}^{(3)}\mathbf{K}'}}-\hat{\epsilon}_{\mathbf{K}^{(3)}\mathbf{K}'\tilde{\mathbf{k}}}\right)^{-1}\right]
\end{aligned} \tag{29}$$

To obtain the relation between dual and lattice self-energy let first express lattice selfenergy as cluster self-energy with additional non-local correction

$$\Sigma_{\omega_n,\mathbf{K},\mathbf{K}',\tilde{\mathbf{k}}} = \Sigma^c_{\omega_n,\mathbf{K}}\delta_{\mathbf{K},\mathbf{K}'} + \bar{\Sigma}_{\omega_n,\mathbf{K},\mathbf{K}',\tilde{\mathbf{k}}}. \tag{30}$$

Using Dyson equation for lattice and cluster self-energy the non-local correction can be expressed as

$$\bar{\Sigma}_{\omega_n,\mathbf{K},\mathbf{K}',\tilde{\mathbf{k}}} = G^{-1}_{\omega_n,\mathbf{K}}\delta_{\mathbf{K},\mathbf{K}'} + \left((\Delta_{\omega_n\mathbf{K}} + \bar{\epsilon}_{\mathbf{K}})_{\delta_{\mathbf{K}\mathbf{K}'}} - \hat{\epsilon}_{\mathbf{K},\mathbf{K}',\tilde{\mathbf{k}}}\right) - \mathbf{G}^{-1}_{\omega_n,\mathbf{K},\mathbf{K}',\tilde{\mathbf{k}}}. \tag{31}$$

Using Eq. 29 we can express lattice Green's function in terms of dual self-energy.

$$\begin{aligned}\mathbf{G}_{\omega_n\mathbf{K}\mathbf{K}'\tilde{\mathbf{k}}} &= \left[\left((\Delta_{\omega_n\mathbf{K}} + \bar{\epsilon}_{\mathbf{K}})_{\delta_{\mathbf{K}\mathbf{K}^{(2)}}} - \hat{\epsilon}_{\mathbf{K}\mathbf{K}^{(2)}\tilde{\mathbf{k}}}\right)^{-1} G^{-1}_{\omega_n\mathbf{K}^{(2)}}\right] \tilde{G}_{\omega_n\mathbf{K}^{(2)}\mathbf{K}^{(3)}\tilde{\mathbf{k}}} \left[G^{-1}_{\omega_n\mathbf{K}^{(3)}}\left((\Delta_{\omega_n\mathbf{K}^{(3)}} + \bar{\epsilon}_{\mathbf{K}^{(3)}})_{\delta_{\mathbf{K}^{(3)}\mathbf{K}^{(4)}}} - \hat{\epsilon}_{\mathbf{K}^{(3)}\mathbf{K}^{(4)}\tilde{\mathbf{k}}}\right)^{-1}\right] \times \\ &\times \left(\mathbb{1} + \left((\Delta_{\omega_n\mathbf{K}^{(4)}} + \bar{\epsilon}_{\mathbf{K}^{(4)}})_{\delta_{\mathbf{K}^{(4)}\mathbf{K}^{(5)}}} - \hat{\epsilon}_{\mathbf{K}^{(4)}\mathbf{K}^{(5)}\tilde{\mathbf{k}}}\right) G_{\omega_n,\mathbf{K}^{(5)}} \tilde{G}^{-1}_{\omega_n\mathbf{K}^{(5)}\mathbf{K}'\tilde{\mathbf{k}}} G_{\omega_n,\mathbf{K}'}\right) = \\ &= \left((\Delta_{\omega_n\mathbf{K}} + \bar{\epsilon}_{\mathbf{K}})_{\delta_{\mathbf{K}\mathbf{K}^{(2)}}} - \hat{\epsilon}_{\mathbf{K}\mathbf{K}^{(2)}\tilde{\mathbf{k}}}\right)^{-1} G^{-1}_{\omega_n\mathbf{K}^{(2)}} \left(\tilde{\Sigma}_{\omega_n,\mathbf{K}^{(2)},\mathbf{K}^{(3)},\tilde{\mathbf{k}}} - \tilde{G}^{-1,(0)}_{\omega_n,\mathbf{K}^{(2)},\mathbf{K}^{(3)},\tilde{\mathbf{k}}}\right)^{-1} (\mathbb{1} + \tilde{\Sigma}_{\omega_n,\mathbf{K}^{(3)},\mathbf{K}',\tilde{\mathbf{k}}} G_{\omega_n,\mathbf{K}'})\end{aligned} \tag{32}$$

And finally the non-local correction to the lattice self-energy can be expressed as

$$\bar{\Sigma}_{\omega_n,\mathbf{K},\mathbf{K}',\tilde{\mathbf{k}}} = \left(\mathbb{1} + \tilde{\Sigma}_{\omega_n,\mathbf{K},\mathbf{K}^{(2)},\tilde{\mathbf{k}}} G_{\omega_n,\mathbf{K}^{(2)}}\right)^{-1} \tilde{\Sigma}_{\omega_n,\mathbf{K}^{(2)},\mathbf{K}',\tilde{\mathbf{k}}}. \tag{33}$$

## III. INTERACTION APPROXIMATION

In order to show the approximation of the interacting term that done in the DCA dual fermions with Laue approximation let's consider the following:

$$\Lambda = \sum_{\mathbf{I}\tilde{\mathbf{i}}} e^{-i(\mathbf{K}_1+\mathbf{K}_3-\mathbf{K}_2-\mathbf{K}_4)\mathbf{I}} e^{-i(\tilde{\mathbf{k}}_1+\tilde{\mathbf{k}}_3-\tilde{\mathbf{k}}_2-\tilde{\mathbf{k}}_4)\tilde{\mathbf{i}}} = \Lambda_{DCA} \sum_{\tilde{\mathbf{i}}} e^{-i(\tilde{\mathbf{k}}_1+\tilde{\mathbf{k}}_3-\tilde{\mathbf{k}}_2-\tilde{\mathbf{k}}_4)\tilde{\mathbf{i}}} \tag{34}$$

with this we can approximate the Fourier transform for grassmann variables:

$$c_{\omega_n,\mathbf{K},\tilde{\mathbf{i}},\sigma} = \frac{1}{\sqrt{N_c}} \sum_{\mathbf{I}} c_{\omega_n,\mathbf{I}+\tilde{\mathbf{i}},\sigma} e^{-i\mathbf{K}\mathbf{I}}, \tag{35}$$

And we can now perform the approximation of lattice action:

$$S = -\sum_{n\mathbf{K}\tilde{\mathbf{k}}\sigma} c^*_{\omega_n,\mathbf{K}+\tilde{\mathbf{k}},\sigma}(i\omega_n + \mu - \epsilon_{\mathbf{K}+\tilde{\mathbf{k}}})c_{\omega_n,\mathbf{K}+\tilde{\mathbf{k}},\sigma} + $$

$$+\frac{U}{N_c^2V^2\beta} \sum_{\substack{n,m,l \\ \mathbf{K}_1\mathbf{K}_2\mathbf{K}_3\mathbf{K}_4 \\ \tilde{\mathbf{k}}_1\tilde{\mathbf{k}}_2\tilde{\mathbf{k}}_3\tilde{\mathbf{k}}_4}} c^*_{\omega_n,\mathbf{K}_1+\tilde{\mathbf{k}}_1,\uparrow} c_{\omega_n+\Omega_l,\mathbf{K}_2+\tilde{\mathbf{k}}_2,\uparrow} c^*_{\omega_m+\Omega_l,\mathbf{K}_3+\tilde{\mathbf{k}}_3,\downarrow} c_{\omega_m,\mathbf{K}_4+\tilde{\mathbf{k}}_4,\downarrow} \Lambda \overset{Apply Eq.\ 34}{=} \tag{36}$$

$$= -\sum_{n\mathbf{K}\tilde{\mathbf{k}}\sigma} c^*_{\omega_n,\mathbf{K}+\tilde{\mathbf{k}},\sigma}(i\omega_n + \mu - \epsilon_{\mathbf{K}+\tilde{\mathbf{k}}})c_{\omega_n,\mathbf{K}+\tilde{\mathbf{k}},\sigma} + \frac{U}{N_c^2V^2\beta} \sum_{\substack{n,m,l \\ \mathbf{K}_1\mathbf{K}_2\mathbf{K}_3\mathbf{K}_4}} \Lambda_{DCA} \sum_{\tilde{\mathbf{i}}} e^{-i(\tilde{\mathbf{k}}_1+\tilde{\mathbf{k}}_3-\tilde{\mathbf{k}}_2-\tilde{\mathbf{k}}_4)\tilde{\mathbf{i}}} \times \tag{37}$$

$$\times \sum_{\tilde{\mathbf{k}}_1\tilde{\mathbf{k}}_2\tilde{\mathbf{k}}_3\tilde{\mathbf{k}}_4} c^*_{\omega_n,\mathbf{K}_1+\tilde{\mathbf{k}}_1,\uparrow} c_{\omega_n+\Omega_l,\mathbf{K}_2+\tilde{\mathbf{k}}_2,\uparrow} c^*_{\omega_m+\Omega_l,\mathbf{K}_3+\tilde{\mathbf{k}}_3,\downarrow} c_{\omega_m,\mathbf{K}_4+\tilde{\mathbf{k}}_4,\downarrow} \tag{38}$$

Consider the last part of the last term keeping in mind Eq. 35:

$$\sum_{\tilde{\mathbf{i}}} e^{-i(\tilde{\mathbf{k}}_1+\tilde{\mathbf{k}}_3-\tilde{\mathbf{k}}_2-\tilde{\mathbf{k}}_4)\tilde{\mathbf{i}}} \sum_{\tilde{\mathbf{k}}_1\tilde{\mathbf{k}}_2\tilde{\mathbf{k}}_3\tilde{\mathbf{k}}_4} c^*_{\omega_n,\mathbf{K}_1+\tilde{\mathbf{k}}_1,\uparrow} c_{\omega_n+\Omega_l,\mathbf{K}_2+\tilde{\mathbf{k}}_2,\uparrow} c^*_{\omega_m+\Omega_l,\mathbf{K}_3+\tilde{\mathbf{k}}_3,\downarrow} c_{\omega_m,\mathbf{K}_4+\tilde{\mathbf{k}}_4,\downarrow} = \tag{39}$$

$$\sum_{\tilde{\mathbf{i}}} \sum_{\tilde{\mathbf{k}}_1} c^*_{\omega_n,\mathbf{K}_1+\tilde{\mathbf{k}}_1,\uparrow} e^{-i\tilde{\mathbf{k}}_1\tilde{\mathbf{i}}} \sum_{\tilde{\mathbf{k}}_2} c_{\omega_n+\Omega_l,\mathbf{K}_2+\tilde{\mathbf{k}}_2,\uparrow} e^{i\tilde{\mathbf{k}}_2\tilde{\mathbf{i}}} \sum_{\tilde{\mathbf{k}}_3} c^*_{\omega_m+\Omega_l,\mathbf{K}_3+\tilde{\mathbf{k}}_3,\downarrow} e^{-i\tilde{\mathbf{k}}_3\tilde{\mathbf{i}}} \sum_{\tilde{\mathbf{k}}_4} c_{\omega_m,\mathbf{K}_4+\tilde{\mathbf{k}}_4,\downarrow} e^{i\tilde{\mathbf{k}}_4\tilde{\mathbf{i}}} \tag{40}$$

Since with approximation Eq. 35

$$c^*_{\omega_n,\mathbf{K}_1,\tilde{\mathbf{i}},\uparrow} = \frac{1}{\sqrt{V}} \sum_{\tilde{\mathbf{k}}_1} c^*_{\omega_n,\mathbf{K}_1+\tilde{\mathbf{k}}_1,\uparrow} e^{-i\tilde{\mathbf{k}}_1\tilde{\mathbf{i}}} \tag{41}$$

we get

$$\sum_{\tilde{\mathbf{i}}}\sum_{\tilde{\mathbf{k}}_1} c^*_{\omega_n,\mathbf{K}_1+\tilde{\mathbf{k}}_1,\uparrow} e^{-i\tilde{\mathbf{k}}_1\tilde{\mathbf{i}}} \sum_{\tilde{\mathbf{k}}_2} c_{\omega_n+\Omega_l,\mathbf{K}_2+\tilde{\mathbf{k}}_2,\uparrow} e^{i\tilde{\mathbf{k}}_2\tilde{\mathbf{i}}} \sum_{\tilde{\mathbf{k}}_3} c^*_{\omega_m+\Omega_l,\mathbf{K}_3+\tilde{\mathbf{k}}_3,\downarrow} e^{-i\tilde{\mathbf{k}}_3\tilde{\mathbf{i}}} \sum_{\tilde{\mathbf{k}}_4} c_{\omega_m,\mathbf{K}_4+\tilde{\mathbf{k}}_4,\downarrow} e^{i\tilde{\mathbf{k}}_4\tilde{\mathbf{i}}} = \tag{42}$$

$$V^2 \sum_{\tilde{\mathbf{i}}} c^*_{\omega_n,\mathbf{K}_1,\tilde{\mathbf{i}},\uparrow} c_{\omega_n+\Omega_l,\mathbf{K}_2,\tilde{\mathbf{i}},\uparrow} c^*_{\omega_m+\Omega_l,\mathbf{K}_3,\tilde{\mathbf{i}},\downarrow} c_{\omega_m,\mathbf{K}_4,\tilde{\mathbf{i}},\downarrow} \tag{43}$$

[1] G. Rohringer, A. Valli, and A. Toschi, Phys. Rev. B **86**, 125114 (2012).
